# Supplementary material for: Beating the Rayleigh Limit Using Two-Photon Interference
Source: arXiv:1803.07096 ancillary file (2018-12-19)
Supplement: Supplementary file 1 [file suppl.pdf]

# Supplemental Material for: Beating the Rayleigh Limit Using Two-Photon Interference

Michał Parniak,[1,2,*] Sebastian Borówka,[1] Kajetan Boroszko,[1] Wojciech Wasilewski,[1,2] Konrad Banaszek,[1,2] and Rafał Demkowicz-Dobrzański[1]

[1]*Faculty of Physics, University of Warsaw, Pasteura 5, 02-093 Warsaw, Poland*
[2]*Centre for Quantum Optical Technologies, Centre of New Technologies, University of Warsaw, Banacha 2c, 02-097 Warsaw, Poland*

## S.I. FI matrix for the two-photon interference protocol

Consider first a situation when two photons to be interfered at the output beamsplitter arrive in the respective spatial modes $|\psi_1\rangle$ and $|\psi_2\rangle$. After interfering them on a balanced beam splitter, we will observe coincidence $c$ (when photons go to different output ports) as well as double events $d$ (when photons go to the same port). If spatial information is taken into account the respective probabilities of observing two photons at positions $(x_1, x_2)$, where position are understood to be measured with respect to the center of the output port in which the photon is found, read:

$$p_{c/d}^{\psi_1,\psi_2}(x_1,x_2) = \frac{1}{4}\bigg(|\psi_1(x_1)\psi_2(x_2)|^2 + |\psi_2(x_1)\psi_1(x_2)|^2 + \\ -/+\ 2\mathcal{V}\mathrm{Re}[\psi_1(x_1)^*\psi_2(x_1)\psi_2(x_2)^*\psi_1(x_2)]\bigg), \quad \text{(S1)}$$

where $\mathcal{V}$ is the visibility of the interferometric setup. Making use of formulas (S1) we can now write the respective probabilities corresponding to the actual two photon state $\rho^{\otimes 2}$ that we deal with in our imaging problem:

$$p_{c/d}(x_1,x_2) = \frac{1}{4}\bigg(p_{c/d}^{x_+,x_+}(x_1,x_2) + p_{c/d}^{x_-,x_-}(x_1,x_2) + \\ p_{c/d}^{x_+,x_-}(x_1,x_2) + p_{c/d}^{x_-,x_+}(x_1,x_2)\bigg). \quad \text{(S2)}$$

According to Eq. (1) in the main text the FI matrix reads:

$$F_{ij} = \frac{1}{2}\int_{-\infty}^{\infty} \mathrm{d}x_1 \mathrm{d}x_2 \left(\frac{\partial_{\theta_i} p_c(x_1,x_2)\partial_{\theta_j} p_c(x_1,x_2)}{p_c(x_1,x_2)} + \\ \frac{\partial_{\theta_i} p_d(x_1,x_2)\partial_{\theta_j} p_d(x_1,x_2)}{p_d(x_1,x_2)}\right), \quad \text{(S3)}$$

where we have introduced the factor 1/2 so that the FI matrix can be regarded as per single photon used. Unfortunately, even for the simple gaussian transfer function, $\psi(x) = (2\pi)^{-1/4}\exp(-x^2/4)$ which we assume in the forthcoming calculations, this formula cannot be calculated analytically. Instead, we perform calculations in successive orders of $\varepsilon$. In ideal case of perfect visibility $\mathcal{V} = 1$, the FI matrix expanded up to the 2-nd order in $\varepsilon$ reads:

$$F_{2\mathrm{P}}^{\mathcal{V}=1} = \begin{bmatrix} 1 - \frac{1}{4}\varepsilon^2 & 0 \\ 0 & \frac{1}{8} + \frac{5}{128}\varepsilon^2 \end{bmatrix} + O(\varepsilon^4), \quad \text{(S4)}$$

while for finite visibility it changes to:

$$F_{2\mathrm{P}}^{\mathcal{V}<1} = \begin{bmatrix} 1 - \frac{1}{4}\varepsilon^2 & 0 \\ 0 & \frac{4-\mathcal{V}^2}{32(1-\mathcal{V}^2)}\varepsilon^2 \end{bmatrix} + O(\varepsilon^4), \quad \text{(S5)}$$

and the last expansion makes sense provided $\frac{\varepsilon^2}{1-\mathcal{V}} \lesssim 1$.

In case we have no access to spatial information, we first need to integrate the respective probability distributions over $x_1$ and $x_2$, which yields

$$p_{c/d} = \frac{1}{4}\left[2 -/+ \mathcal{V}\left(1 + e^{-\frac{\varepsilon^2}{4}}\right)\right]. \quad \text{(S6)}$$

Clearly, ignoring the spatial information we do not have access to information about the centroid position $x_c$. The resulting FI for estimation of the $\varepsilon$ parameter can be calculated exactly:

$$(F_{2\mathrm{P}}^{\text{no spatial}})_{22} = \frac{\varepsilon^2\mathcal{V}^2}{8\left[(2-\mathcal{V})e^{\varepsilon^2/4} - \mathcal{V}\right]\left[(2+\mathcal{V})e^{\varepsilon^2/4} + \mathcal{V}\right]} \\ \approx \begin{cases} \frac{1}{8} - \frac{5}{128}\varepsilon^2 & \mathcal{V} = 1 \\ \frac{\mathcal{V}^2\varepsilon^2}{32(1-\mathcal{V}^2)} & \mathcal{V} < 1 \end{cases} + O(\varepsilon^4). \quad \text{(S7)}$$

Since all FI matrices for the problem considered are diagonal, we can identify the diagonal entries with bounds on inverse of the variance of estimating the respective parameters.

## S.II. Photon pair source

The spectrally degenerate $|hv\rangle$ photon pairs at 798 nm are generated by driving a quasi-phase matched spontaneous parametric down-conversion in 5-mm-long PP-KTP crystal with poling period of 9.2 $\mu$m with a 399 nm continous-wave diode laser. To maintain spectral degeneracy of the photon pairs the crystal is kept at a constant temperature of 23.0°C and the photons are subsequently filtered with a 1-nm broad bandpass filter. A single spatial mode is selected using a single-mode fiber which directs the photon pairs to the main part of experimental setup presented in Fig. 2(a).

### S.III. Generation of the $\rho^{\otimes 2}$ state

We direct the photons generated in type-II spontaneous parametric down-conversion process into the interferometer in a Mach-Zehnder configuration [see Fig. 2(a) in the main text]. By positioning the retro-reflectors inside each arm we set each photon in a specific mode with a precisely controlled offset from the principal axis—note that reconfiguring is necessary even for a fixed $\varepsilon$ as we want to reproduce within our setup the results corresponding to the mixed state $\rho^{\otimes 2}$ which is a mixture of four different pure states. The photons are then directed through standard common-path polarization Hong-Ou-Mandel interferometer [S1] after which we separate each output port (which correspond to measurement in the rotated $\{|a\rangle,\ |d\rangle\}$ polarization basis) into two beams. Finally, we perform spatially-resolved single-photon detection with the I-sCMOS camera using four distinct regions as each beam is split to allow auto-coincidence (double events) detection within the Hanbury Brown-Twiss scheme. With the setup we may generate the $\rho^{\otimes 2}$ state for a set $\varepsilon$ by positioning the retro-reflectors for equal periods of time in each configuration (i.e. both modes populated by one photon or each mode populated by two photons). Importantly, changing position of retro-reflectors keeps a constant delay between photons allowing good temporal overlap of two photons and thus ensuring their indistinguishability in the temporal degree of freedom.

### S.IV. Data analysis and experimental estimation

For the experimental points in Figs. 2(c) and 2(d) we used 1000 detected coincidences and double events and repeated the ML estimation for each dataset to obtain both the precision and its errorbar corresponding to one standard deviation. Since not all detected double events are used in the estimation procedure (i.e we only consider double events in which two photons are registered in separated regions of the camera) the number of resources used is estimated as $N = 2N_c + 4N_d$. For the theoretical curves we go beyond the derived expansions and provide precision obtained from the numerically evaluated FI.

### S.V. Spatially-resolved detection

Detection of single photons in each of the four regions is performed using a single self-assembled I-sCMOS camera. The camera consists of a microchannel plate (MCP) based image intensifier (Hamamatsu V7090D), a relay lens and an sCMOS camera (Zyla), operated at 4.5 kHz frame rate. The image intensifier MCP is gated using a Photek GM10-50B gating module with 150 ns gate time. Electron avalanches in the MCP excite a phosphor screen (type P43) which is subsequently imaged at the sCMOS sensor. Since a single phosphor emission event (a localized flash) lasts for $\sim$ 1 ms it is registered on up to 20 sCMOS camera frames - note that this issue can be easily mitigated with a phosphor screen characterized by a shorter decay time as in [S2] if faster experimental rates are required. Here, we post-select only true coincidences by rejecting 20 frames after a phosphor screen flash is observed. Real-time software localizes the flashes and then their positions are stored as photon coordinates, subsequently binned into effective pixels. Data is processed by sorting photons into four regions of interest (A, B, C and D) and analyzing all possible coincidences between the regions. Coincidences within one region are not counted due to deleterious cross-talk, which can however be mitigated via elaborate post-processing techniques [S3]. To maintain high coincidence-to-accidental ratio (or equivalently high value of cross correlation function $g^{(2)}_{hv}$) we set the probability to detect a single photon per camera frame of $5 \times 10^{-4}$ by using approx. 1 mW of blue laser power, resulting in coincidence probability of $1.7 \times 10^{-5}$ compared with an estimate of $2.5 \times 10^{-7}$ accidental coincidence probability. Efficiency of the entire system nets to approx. 3.5% and the dark count probability is $< 10^{-5}$ per single region of interest.

---

* michal.parniak@fuw.edu.pl

[S1] M. Jachura, R. Chrapkiewicz, R. Demkowicz-Dobrzański, W. Wasilewski, and K. Banaszek, Nat. Commun. **7**, 11411 (2016).
[S2] M. Parniak, M. Dąbrowski, M. Mazelanik, A. Leszczyński, M. Lipka, and W. Wasilewski, Nat. Commun. **8**, 2140 (2017).
[S3] M. Lipka, M. Parniak, and W. Wasilewski, Appl. Phys. Lett. **112**, 211105 (2018).
